# Supplementary material for: MACARONS: Mapping And Coverage Anticipation with RGB Online Self-Supervision
Source: arXiv:2303.03315 source file (2023-06-13)
Supplement: Supplementary file 1 [file occupancy.tex]

\begin{figure*}
  \centering
  \begin{subfigure}{0.23\linewidth}
    %\fbox{\rule{0pt}{0.5in} \rule{.9\linewidth}{0pt}}
    \includegraphics[width=\linewidth]{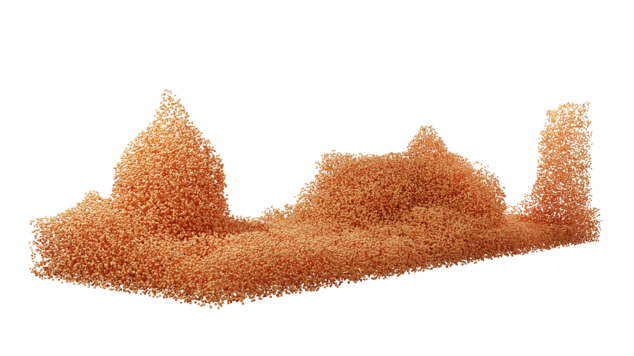}
    \caption{Pisa Cathedral}
  \end{subfigure}
  \hfill
  \begin{subfigure}{0.23\linewidth}
    % \fbox{\rule{0pt}{0.5in} \rule{.9\linewidth}{0pt}}
    \includegraphics[width=\linewidth]{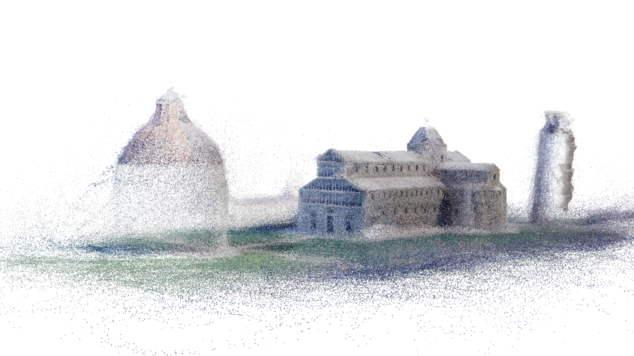}
    \caption{Pisa Cathedral}
  \end{subfigure}
  \hfill
  \begin{subfigure}{0.23\linewidth}
    %\fbox{\rule{0pt}{0.5in} \rule{.9\linewidth}{0pt}}
    \includegraphics[width=\linewidth]{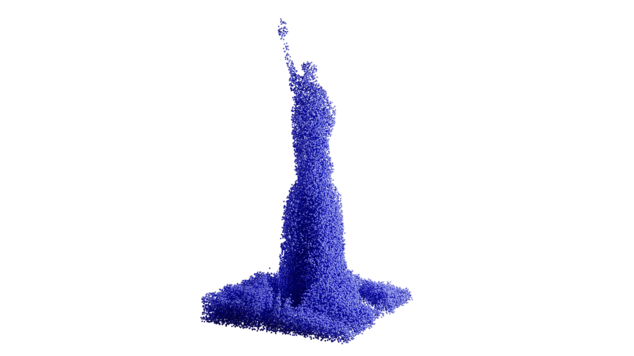}
    \caption{Statue of Liberty}
  \end{subfigure}
  \hfill
  \begin{subfigure}{0.23\linewidth}
    %\fbox{\rule{0pt}{0.5in} \rule{.9\linewidth}{0pt}}
    \includegraphics[width=\linewidth]{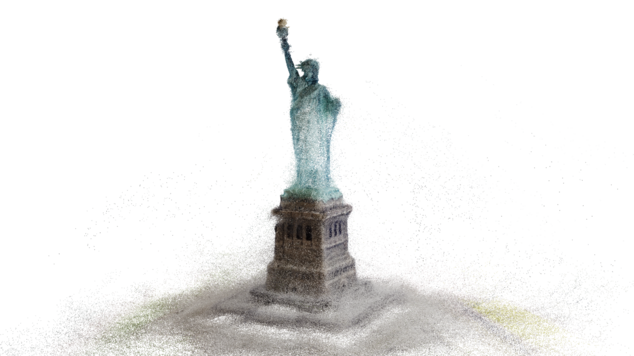}
    \caption{Statue of Liberty}
  \end{subfigure}
  \hfill \\
  \begin{subfigure}{0.23\linewidth}
    %\fbox{\rule{0pt}{0.5in} \rule{.9\linewidth}{0pt}}
    \includegraphics[width=\linewidth]{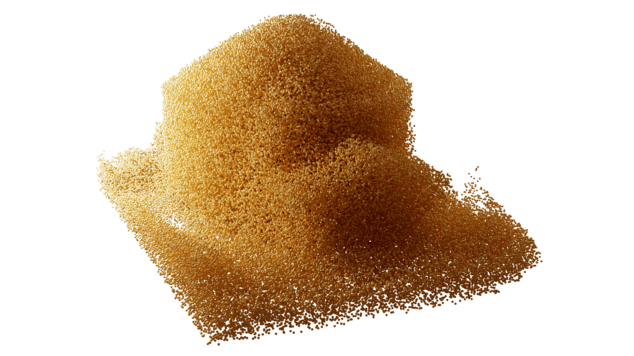}
    \caption{Pantheon}
  \end{subfigure}
  \hfill
  \begin{subfigure}{0.23\linewidth}
    %\fbox{\rule{0pt}{0.5in} \rule{.9\linewidth}{0pt}}
    \includegraphics[width=\linewidth]{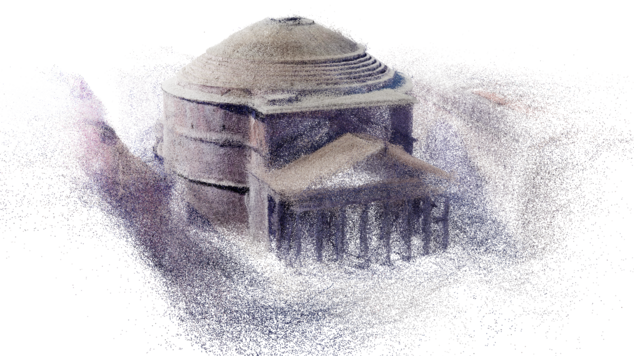}
    \caption{Pantheon}
  \end{subfigure}
  \hfill
    \begin{subfigure}{0.23\linewidth}
    % \fbox{\rule{0pt}{0.5in} \rule{.9\linewidth}{0pt}}
    \includegraphics[width=\linewidth]{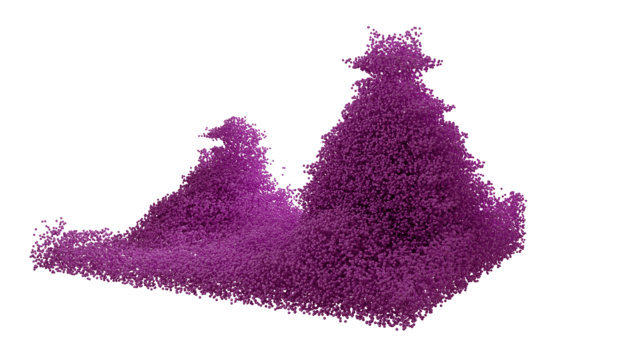}
    \caption{Fushimi Castle}
  \end{subfigure} 
  \hfill
  \begin{subfigure}{0.23\linewidth}
    %\fbox{\rule{0pt}{0.5in} \rule{.9\linewidth}{0pt}}
    \includegraphics[width=\linewidth]{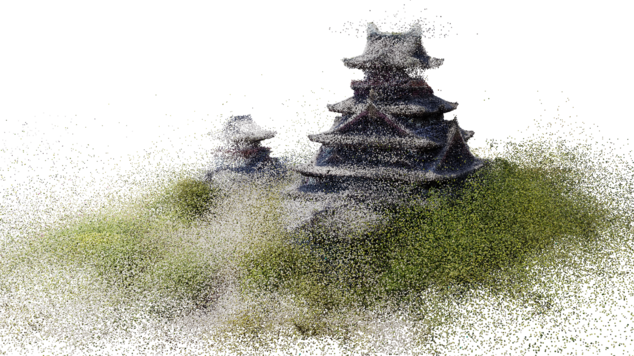}
    \caption{Fushimi Castle}
  \end{subfigure} \\
  \begin{subfigure}{0.23\linewidth}
    % \fbox{\rule{0pt}{0.5in} \rule{.9\linewidth}{0pt}}
    \includegraphics[width=\linewidth]{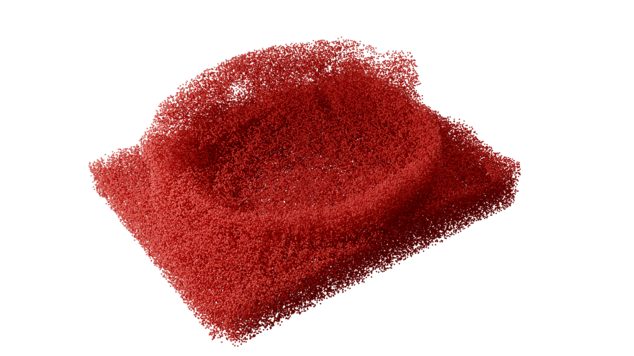}
    \caption{Colosseum}
  \end{subfigure}
  \hfill
    \begin{subfigure}{0.23\linewidth}
    %\fbox{\rule{0pt}{0.5in} \rule{.9\linewidth}{0pt}}
    \includegraphics[width=\linewidth]{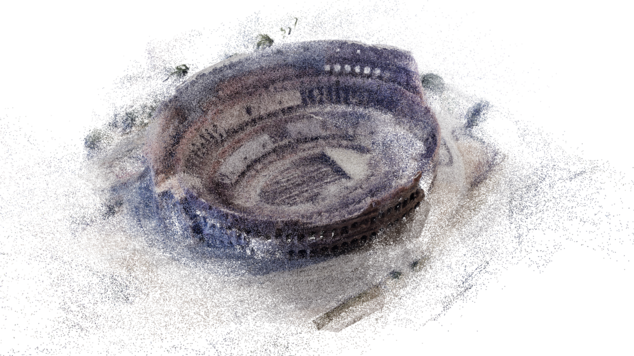}
    \caption{Colosseum}
  \end{subfigure}
  \hfill
  \begin{subfigure}{0.23\linewidth}
    %\fbox{\rule{0pt}{0.5in} \rule{.9\linewidth}{0pt}}
    \includegraphics[width=\linewidth]{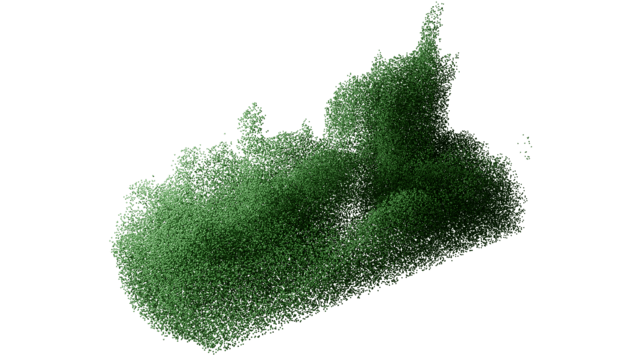}
    \caption{Neuschwanstein Castle}
  \end{subfigure}
  \hfill
    \begin{subfigure}{0.23\linewidth}
    %\fbox{\rule{0pt}{0.5in} \rule{.9\linewidth}{0pt}}
    \includegraphics[width=\linewidth]{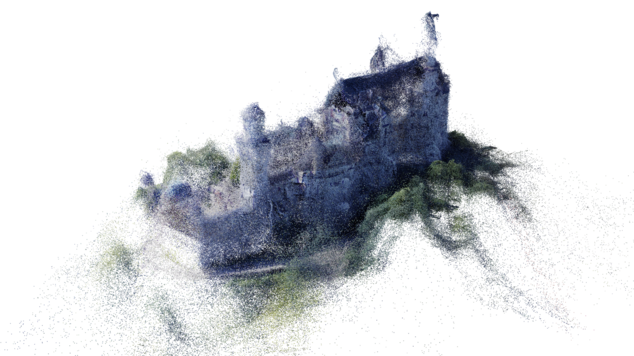}
    \caption{Neuschwanstein Castle}
  \end{subfigure}
  \caption{{\bf Volume occupancy fields computed with our approach MACARONS.} Our model updates the volume occupancy field in real time during exploration: For several scene, we show here the volume occupancy after 100 NBV iterations (left), as well as the final reconstructed surface for comparison (right).% The model has been trained on a set of previous scenes; all weights  are frozen and we only perform inference computation. The first four rows depict scenes that were already seen by the model during its online, self-supervised training. The last two rows depicts scenes the model has never seen before.
  }
  \label{fig:supp-mat-occupancy}
\end{figure*}
