# Supplementary material for: MACARONS: Mapping And Coverage Anticipation with RGB Online Self-Supervision
Source: arXiv:2303.03315 source file (2023-06-13)
Supplement: Supplementary file 3 [file rgb_depth.tex]

\begin{figure}
  \centering

  \begin{subfigure}{0.23\linewidth}
    \fbox{\rule{0pt}{0.5in} \rule{.9\linewidth}{0pt}}
    %\includegraphics[width=\linewidth]{images/occupancy_probability/pantheon_t0.png}
    % \caption{Statue of Liberty.}
    %\label{fig:occ-b}
  \end{subfigure}
  \hfill
  \begin{subfigure}{0.23\linewidth}
    \fbox{\rule{0pt}{0.5in} \rule{.9\linewidth}{0pt}}
    %\includegraphics[width=\linewidth]{images/occupancy_probability/pantheon_t1.png}
    % \caption{Statue of Liberty.}
    %\label{fig:occ-c}
  \end{subfigure}
  \hfill
  \begin{subfigure}{0.23\linewidth}
    \fbox{\rule{0pt}{0.5in} \rule{.9\linewidth}{0pt}}
    %\includegraphics[width=\linewidth]{images/occupancy_probability/pantheon_t2.png}
    % \caption{Statue of Liberty.}
    %\label{fig:occ-d}
  \end{subfigure}
  \hfill
    \begin{subfigure}{0.23\linewidth}
    \fbox{\rule{0pt}{0.5in} \rule{.9\linewidth}{0pt}}
    %\includegraphics[width=\linewidth]{images/occupancy_probability/pantheon_comparison.png}
    % \caption{Pisa Cathedral.}
    %\label{fig:occ-a}
  \end{subfigure}\\
  \begin{subfigure}{0.23\linewidth}
    \fbox{\rule{0pt}{0.5in} \rule{.9\linewidth}{0pt}}
    \caption{\scriptsize $I_{t-2}$}
    %\label{fig:occ-b-bis}
  \end{subfigure}
    \hfill
  \begin{subfigure}{0.23\linewidth}
    \fbox{\rule{0pt}{0.5in} \rule{.9\linewidth}{0pt}}
    % \includegraphics[width=\linewidth]{images/occupancy_probability/pisa_t1.png}
    % \caption{Statue of Liberty.}
    \caption{\scriptsize $I_{t-1}$}
    % \label{fig:occ-c-bis}
  \end{subfigure}
  \hfill
  \begin{subfigure}{0.23\linewidth}
    \fbox{\rule{0pt}{0.5in} \rule{.9\linewidth}{0pt}}
    % \includegraphics[width=\linewidth]{images/occupancy_probability/pisa_t2.png}
    % \caption{Statue of Liberty.}
    \caption{\scriptsize $I_t$}
    % \label{fig:occ-d-bis}
  \end{subfigure}
  \hfill
  \begin{subfigure}{0.23\linewidth}
    \fbox{\rule{0pt}{0.5in} \rule{.9\linewidth}{0pt}}
    \caption{\scriptsize $d_t$}
    % \label{fig:occ-a-bis}
  \end{subfigure}
%   \caption{{\bf Volume occupancy probability field of large 3D structures.} The second module of MACARONS predicts and updates in real-time a volume occupancy probability field (right) from the reconstructed surface points (left).}
  \caption{\textbf{Depth prediction from a sequence of RGB images by our model MACARONS.} At time step $t$, the depth prediction module of MACARONS takes as input the RGB images $I_t, I_{t-1}, ..., I_{t-m}$ to predict the depth map $d_t$. We take $m=2$ in our experiments.}
  \label{fig:supp-mat-rgb-depth}
\end{figure}
